# Supplementary material for: A surprisal oracle for when every layer counts
Source: arXiv:2412.03098 source file (2024-12-04)
Supplement: Supplementary file 1 [file appendix1_24.tex]

 



%%% blimp supplement

%\begin{table*}[th!]
%    \centering
%    \resizebox{\textwidth}{!}{% 
%    $\begin{tabular}{l R{1.2cm} R{1.2cm} R{1.2cm} R{1.2cm} R{1.2cm} R{1.2cm} R{1.2cm} R{1.2cm}}
%    \toprule
%& \multicolumn{4}{c}{Submitted ELC-BERT ACLM models}& \multicolumn{4}{c}{Baselines} \\\cmidrule{6-9}
%& & & & & \multicolumn{2}{c}{Ours} & \multicolumn{2}{c}{Official} \\\cmidrule{6-7}\cmidrule{7-9}
%  &	Model 1 &	Model 2 &	Model 3 &	Model 4 &	Batch-512 & Batch-64/B32 & BabyLlama & LTG-BERT\\
%\midrule
%blimp supplement & & & & & & & & \\
%\midrule
%hypernym                                       &&&&&&0.5439\\
%qa congruence easy                             &&&&&&0.5156\\
%qa congruence tricky                             &&&&&&0.4485\\
%subject aux inversion                            &&&&&&0.4184\\
%turn taking                                      &&&&&&0.5286\\

%\end{tabular}$
    %\caption{Accuracy scores of the zero-shot evaluation on the BLiMP dataset. All models were trained on the data for the strict-small track. QA Cong. means QA Congruence. Inv. means inversion.}
%}
%\end{table*}

%%% Blimp filtered

%\begin{table*}[th!]
%    \centering
 %   \resizebox{\textwidth}{!}{% 
%    \begin{tabular}{l R{1.2cm} R{1.2cm} R{1.2cm} R{1.2cm} R{1.2cm} R{1.2cm} R{1.2cm} R{1.2cm}}
%    \toprule
%& \multicolumn{4}{c}{Submitted ELC-BERT ACLM models}& \multicolumn{4}{c}{Baselines} \\\cmidrule{6-9}
%& & & & & \multicolumn{2}{c}{Ours} & \multicolumn{2}%{c}{Official} \\\cmidrule{6-7}\cmidrule{7-9}
  %&	Model 1 &	Model 2 &	Model 3 &	Model 4 %&	Batch-512 & Batch-64/B32 & BabyLlama & LTG%-BERT\\
%\midrule 
%adjunct island                                     %&&&&&&0.5022\\
%anaphor gender agreement                           %&&&&&&0.5232\\
%anaphor number agreement                           %&&&&&&0.4941\\
%animate subject passive                            %&&&&&&0.5117\\
%animate subject trans                              %&&&&&&0.5417\\
%causative                                          %&&&&&&0.4352\\
%complex NP island                                  %&&&&&&0.4291\\
%coord. struc. constraint complex left %branch&&&&&&0.5199\\
%coord. struc. constraint object extraction  %&&&&&&0.4584\\
%det. noun agreement 1                        %&&&&&&0.4919\\
%det. noun agreement 2                        %&&&&&&0.4952\\
%det. noun agreement irregular 1              %&&&&&&0.5492\\
%det. noun agreement irregular 2              %&&&&&&0.4390\\
%det. noun agreement with adj 2               %&&&&&&0.4708\\
%det. noun agreement with adj irregular 1     %&&&&&&0.5251\\
%det. noun agreement with adj irregular 2     %&&&&&&0.4536\\
%det. noun agreement with adjective 1         %&&&&&&0.4887\\
%distractor agreement relational noun               %&&&&&&0.5508\\
%distractor agreement relative clause               %&&&&&&0.4868\\
%drop argument                                      %&&&&&&0.4511\\
%ellipsis n bar 1                                   %&&&&&&0.4875\\
%ellipsis n bar 2                                   %&&&&&&0.4372\\
%existential there object raising                   %&&&&&&0.5369\\
%existential there quantifiers 1                    %&&&&&&0.6871\\
%existential there quantifiers 2                    %&&&&&&0.5357\\
%existential there subject raising                  %&&&&&&0.5195\\
%expletive it object raising                        %&&&&&&0.5086\\
%inchoative                                         %&&&&&&0.5018\\
%intransitive                                       %&&&&&&0.4965\\
%irregular past participle adjectives               %&&&&&&0.5036\\
%irregular past participle verbs                    %&&&&&&0.5117\\
%irregular plural subject verb agreement 1          %&&&&&&0.4863\\
%irregular plural subject verb agreement 2          %&&&&&&0.5314\\
%left branch island echo question                   %&&&&&&0.2904\\
%left branch island simple question                 %&&&&&&0.5436\\
%matrix question npi licensor present               %&&&&&&0.3950\\
%npi present 1                                      %&&&&&&0.0473\\
%npi present 2                                      %&&&&&&0.0635\\
%only npi licensor present                          %&&&&&&0.8084\\
%only npi scope                                     %&&&&&&0.3955\\
%passive 1                                          %&&&&&&0.4893\\
%passive 2                                          %&&&&&&0.5138\\
%principle A c command                              %&&&&&&0.5264\\
%principle A case 1                                 %&&&&&&0.3125\\
%principle A case 2                                 %&&&&&&0.5257\\
%principle A domain 1                               %&&&&&&0.2888\\
%principle A domain 2                               %&&&&&&0.4918\\
%principle A domain 3                               %&&&&&&0.4973\\
%principle A reconstruction                         %&&&&&&0.4571\\
%regular plural subject verb agreement 1            %&&&&&&0.4955\\
%regular plural subject verb agreement 2            %&&&&&&0.5132\\
%sentential negation npi licensor present           %&&&&&&0.3830\\
%sentential negation npi scope                      %&&&&&&0.4960\\
%sentential subject island                          %&&&&&&0.5369\\
%superlative quantifiers 1                          %&&&&&&0.4505\\
%superlative quantifiers 2                          
%&&&&&&0.4594\\
%tough vs raising 1                                 %&&&&&&0.5084\\
%tough vs raising 2                                 %&&&&&&0.5098\\
%transitive                                         %&&&&&&0.4781\\
%wh island                                          %&&&&&&0.5979\\
%wh questions object gap                            %&&&&&&0.4529\\
%wh questions subject gap                           %&&&&&&0.5312\\
%wh questions subject gap long distance             %&&&&&&0.5508\\
%wh vs that no gap                                  %&&&&&&0.4820\\
%wh vs that no gap long distance                    %&&&&&&0.7520\\
%wh vs that with gap                                %&&&&&&0.3667\\
%wh vs that with gap long distance                  %&&&&&&0.2857\\
%    \end{tabular}}
    %\caption{Accuracy scores of the zero-shot evaluation on the BLiMP dataset. All models were trained on the data for the strict-small track. QA Cong. means QA Congruence. Inv. means inversion.}
%\end{table*}
